# Supplementary material for: ShiftAddAug: Augment Multiplication-Free Tiny Neural Network with Hybrid Computation
Source: arXiv:2407.02881 source file (2024-07-03)
Supplement: Supplementary file 1 [file 6_appendix.tex]

\section{The specific meaning of method} \label{section:method_meaning}
    \begin{figure}[h]
        \centering
        \includegraphics[width=0.6\linewidth]{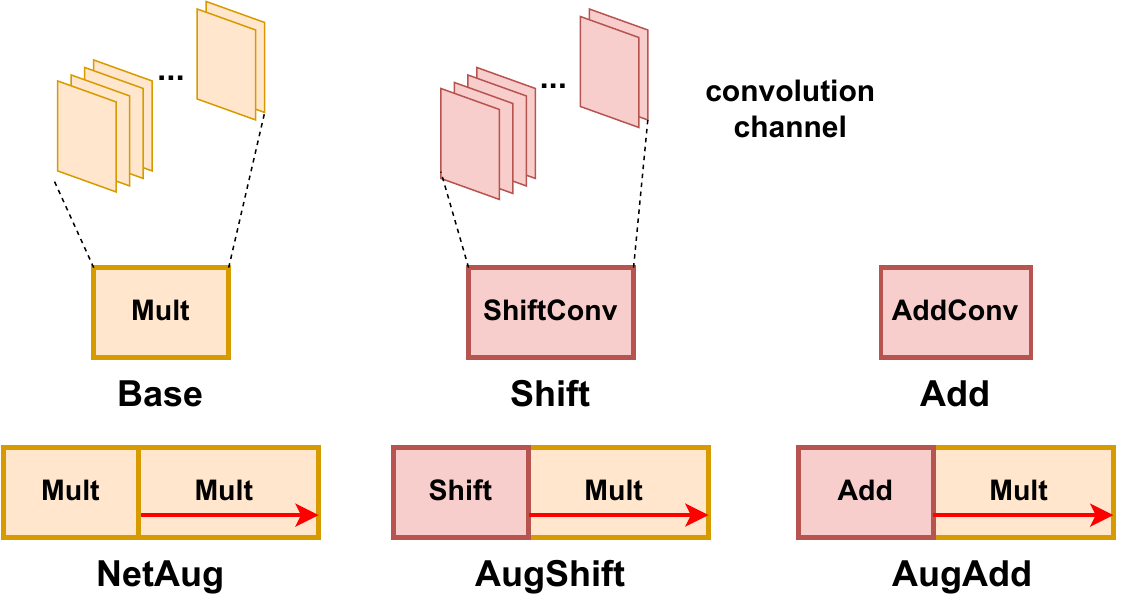}
        % \vspace{-1em}
        \caption{Schematic diagram of each method.}
        \label{fig:method_diagram}
        \vspace{-1em}
    \end{figure}
    
    \begin{itemize}
        \item Base: directly trained multiplicative NN.
        \item NetAug: multiplicative NN with multiplicative augmentation.
        \item Shift: directly trained shift-only-NN with ShiftConv in DeepShift\cite{elhoushi2021deepshift}.
        \item AugShift: ShiftConv with multiplicative augmentation.
        \item Add: directly trained add-NN with AddConv in AdderNet\cite{chen2021addernet}.
        \item AugAdd: AddConv with multiplicative augmentation.
        \item ShiftAddAug (Mult-free): results of neural architecture search with shift/add operator only
        \item ShiftAddAug: results of neural architecture search with shift/add/mult. operator
    \end{itemize}

\section{More results on classification tasks} \label{section:moreClassifyResults}

    \input{tables/moreClassifyDatasets_moreResults}
    Due to the poor training efficiency of the AddConv operator, we mainly focus on ShiftConv when training on these datasets.

\section{More Ablation Study of Heterogeneous Weight Sharing} \label{section:ablation_HWS}

    \textbf{Is weight sharing important?} HWS is needed because we share weights during training, but the weight distributions of different operators are inconsistent. Specifically, we reorder important weights to the target model at the end of each epoch. To illustrate the necessity of our proposed HWS, we first demonstrate the importance of weight sharing for our augmented training. The result in Tab. \ref{tab:ablation_shiftaug} tells that model trained directly based on ShiftConv will have a little accuracy drop. If we augment it with Shift, it yields an average accuracy improvement of \hrup{1.02\%}. But if we don't share weights, i.e. don't reorder important weights in target part, it would only achieve a little improvement. Therefore, weight sharing is one of the key technologies of augmented training.
    \input{tables/rebuttal_weightshare}

    \textbf{The difference from ShiftAddNas.} When encountering the issue of weight tearing, we first thought of the solution in ShiftAddNAS\cite{you2022shiftaddnas}. However, when we applied it, the training loss didn't converge, which made us believe that the method is not suitable for our training situation and it is difficult to compare performance. ShiftAddNas sorts the values of weights, dividing them into $n$ groups from bottom to top, and then sets $n$ learnable parameters to scale the weight values within each group, then put them back. Such an approach naturally leads to a disconnect in the distribution of weights. Our HWS strategy uses fully connected to remap the Conv kernel and use Equ.\ref{equ:weightRemap} to handle different weight distributions.  The obtained result is only added to the original weight as a bias, rather than applied directly. We use directly trained multiplicative and multiplication-free Conv weights as datasets to train the FC layer here, and freeze it in augmented training. 
    
    We believe that our method has better training stability than ShiftAddNas. As shown in Tab.\ref{tab:rebuttal_convergence}, the ShiftAddNas method and direct mapping with learnable Linear will make it unable to train.

    \vspace{1em}

    \begin{table}[ht]
    \vspace{-1.0em}
  \setlength{\tabcolsep}{4pt}
  \caption{The ablation study of different method for HWS}
  \centering
  % \caption{??????????????????????????}
   % increase vertical spacing
  \resizebox{\linewidth}{!}{
    \begin{tabular}{c|c|c|c|c|c}
    \hline
    \hline
    \textbf{Method} & \textbf{MobileNetV2 w0.35} & \textbf{MobileNetV3 w0.35} & \textbf{MCUNet} & \textbf{ProxylessNAS w0.35} & \textbf{MobileNet-tiny} \\
    
    \hline
    \hline

    ShiftAddNAS & Nan & Nan & Nan & Nan & Nan \\

    Linear remap & Nan & Nan & Nan & Nan & Nan \\

    KL-loss only & 69.84 & 69.98 & 71.12 & 70.52 & 68.70 \\

    Linear + skip connect + freeze & 71.02 & 72.70 & 74.44 & 72.99 & 71.08 \\

    \hline
    
    \textbf{Ours} & 71.83 & 73.37 & 74.59 & 73.86 & 71.89 \\
    \hline
    \hline
    \end{tabular}%
    }
  \label{tab:rebuttal_convergence}%
  \vspace{0.0em}
\end{table}%

    \textbf{Is HWS a parameterization trick that can directly improve the target model?} We designed this ablation study to demonstrate that our HWS remapping method does not improve the accuracy of multiplication-free NNs by itself. On the contrary, it slightly damages the accuracy of the model.  This kind of remapping is only a compensation method for different weight distributions, and will not produce gain for directly trained multiplication-free NNs.

    \input{tables/rebuttal_woAug}

\section{Segmentation effect comparison} \label{section:ablation_iris}
    
    The segmentation of iris, pupil and sclera plays an important role in eye tracking in VR devices. To cope with this task, it is highly cost-effective to use fast and energy-efficient multiplication-free neural networks on such devices. OpenEDS\cite{palmero2020openeds2020} is a large scale dataset of eye-images captured using a virtual-reality (VR) devices. We use it as an example of application. 
    
    In order to achieve the segmentation function, we replace the classification head of the original model with transposed convolution, and use augmentation for the backbone part only. We train each model from scratch for 100 epochs with a base learning rate of 0.001 and batch size of 8.

    From the results shown in Fig. \ref{fig:iris_result}, we can see that the model trained with augmentation will have fewer abnormal segmentation areas.
    
    \begin{figure}[h]
        \centering
        \includegraphics[width=0.9\linewidth]{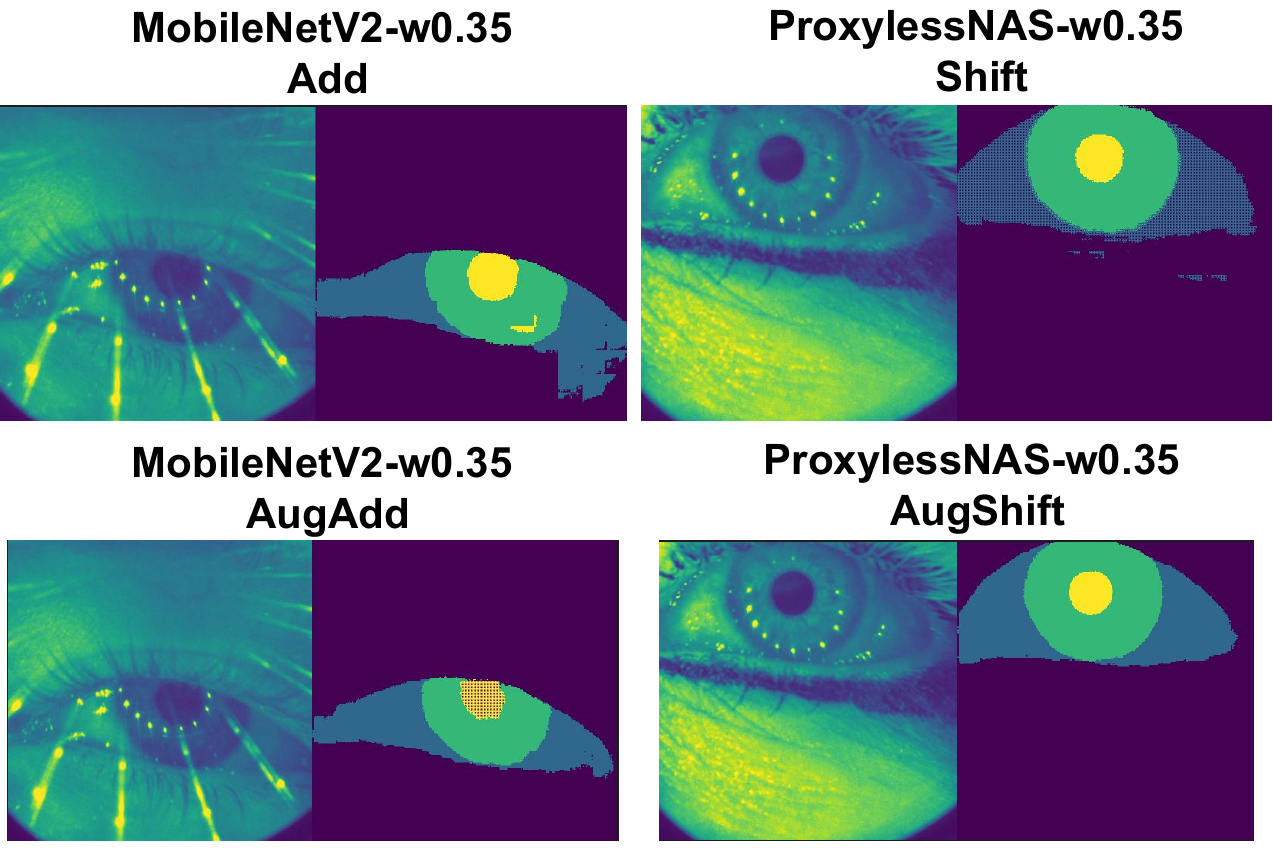}
        \vspace{-1.0em}
        \caption{ShiftAddAug on OpenEDS.}
        \label{fig:iris_result}
        \vspace{-1.0em}
    \end{figure}

\section{Latency on general GPUs with TVM} \label{section:latency_tvm}

    In most experiments, we follow ShiftAddNAS\cite{you2022shiftaddnas} and use the simulator to evaluate latency and energy cost, because multiplication-free operators require special hardware design to take full advantage. But considering that general GPUs are widely used computing devices, we also tested the speed of our model through TVM\cite{chen2018tvm} on GPU.

    Since our method does not involve modification of the operator itself and does not generate any inference overhead. These results are also applicable for models trained directly with Deepshift and AdderNet. Like the results in ShiftAddVit\cite{you2023shiftaddvit}, the efficiency of the multiplication-free operator is verified again. But this has nothing to do with the effectiveness of our proposed method.

    We use TVM to build the shift/add models and deploy them on RTX 3090. Batch\_size = 8 for latency testing (ms). The baseline multiplicative model is evaluated in Pytorch. The input resolution is 160.

    \begin{table}[htbp]
  \setlength{\tabcolsep}{4pt}
  \centering
  % \vspace{-1.5em}
  \caption{Latency (ms) comparison with multiplication model on RTX 3090.}
   % increase vertical spacing
  \resizebox{0.75\linewidth}{!}{
    \begin{tabular}{c|c|c|c|c|c}
    \hline
    \hline
    \textbf{Method} & \textbf{MobileNetV2 w0.35} & \textbf{MobileNetV3 w0.35} & \textbf{MCUNet} & \textbf{ProxylessNAS w0.35} & \textbf{MobileNet-tiny} \\
    
    \hline
    \hline

    Baseline & 4.65 & 5.42 & 4.75 & 5.38 & 4.73 \\

    % \hline

    Shift & 1.35 & 2.24 & 1.55 & 1.62 & 1.36 \\

    % \hline

    Add & 3.76 & 4.93 & 4.68 & 5.19 & 3.864 \\
        
    \hline
    \hline
    \end{tabular}%
    }
  \label{tab:rebuttal_TVM}%
  \vspace{-0.5em}
\end{table}%

\section{Ablation Study of Training Settings}

    \begin{figure}[h]
        \centering
        \includegraphics[width=0.4\linewidth]{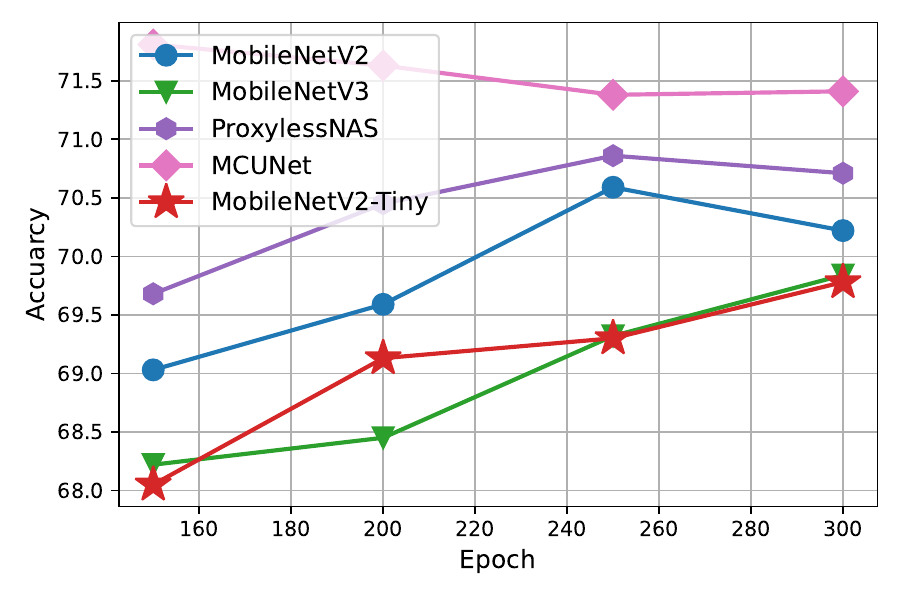}
        \vspace{-1.5em}
        \caption{Baseline accuracy with training epochs.}
        \label{fig:ablation_epoch}
        \vspace{0.0em}
    \end{figure}

    More training epochs can improve accuracy as shown in Fig.\ref{fig:ablation_epoch}. However, training for too long may produce overfitting on the augmented model and require more training time. As a trade-off, we choose to train 250 epochs on the datasets such as CIFAR-10/100. A similar ablation study on ImageNet can be found in NetAug\cite{NetAug}.

    \begin{figure}[h]
        \centering
        \includegraphics[width=0.4\linewidth]{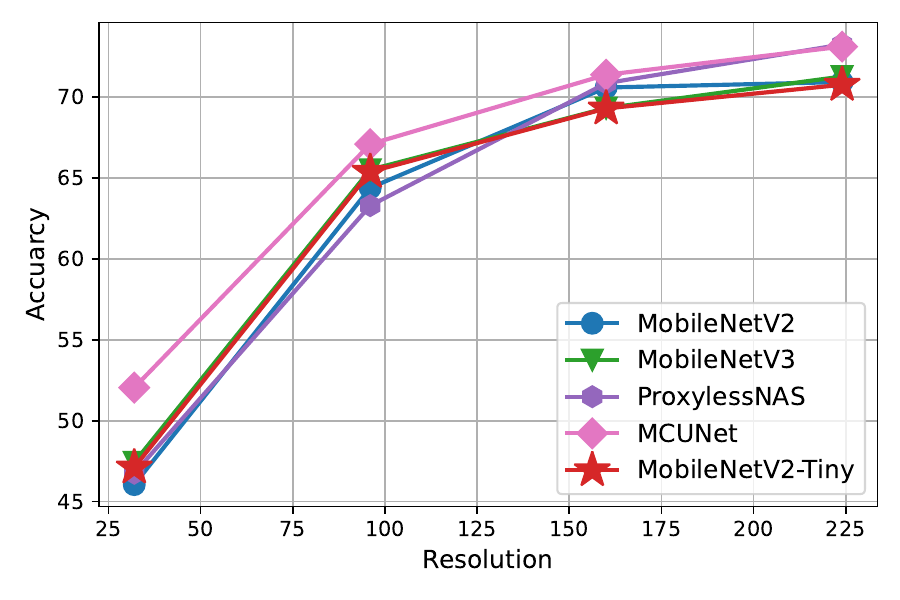}
        \vspace{-1.5em}
        \caption{Baseline accuracy with different input resolution.}
        \label{fig:ablation_res}
        \vspace{0em}
    \end{figure}

    As shown in Fig. \ref{fig:ablation_epoch}, higher resolution improves the accuracy but introduces more computation. We decided that all inputs should be resized to 160 during training and inference. Our model has a smaller capacity, allowing it to consume less energy than previous work with larger resolutions. This setting also means our experimental conclusions won't be limited to low-resolution datasets. 

\section{More Training Details} \label{section:train_setting}

    For ImageNet, we train models with batch size 768 on 6 GPUs. We use the SGD optimizer with Nesterov momentum of 0.9 and weight decay 4e-5. The initial learning rate is 0.15 and gradually decreases to 0 following the cosine schedule. Label smoothing is used with a factor of 0.1. We train 150 epochs with the multiplicative model and then finetune 100 epochs for the Shift model with the same setting. The models with AddConv are trained from scratch for 300 epochs.

    For CIFAR10, we use pre-trained weights from CIFAR100 with original Conv and finetune 100 epochs for the Shift model. The models with AddConv are trained from scratch for 300 epochs on 2 GPUs. For other datasets, we load pre-trained weights from ImageNet and finetune with the same settings.

    For the neural architecture search, we changed the model structures based on MCUNet and MobileNetV3 and pre-explored 100 model structures that met the hardware requirements. Energy consumption and latency can be easily obtained. We start training from the model that meets the conditions with the largest computational amount. Evolutionary algorithms are then used to explore other model structures. Any setting that exceeds the hardware limit will be stopped early and output 0\% accuracy as a penalty. We trained them for 30 epochs for quick exploration and trained the top 10 for the full 300-epoch training.

    For ShiftConv, its weights are quantized to 5 bits, and activations are quantized to 16 bits during calculation. For AddConv, all calculations are performed under 16 bits.

    For HWS, we take the weights on the convolution kernel as input into the FC. The FC has a hidden layer enlarged by a factor of 8. Then values goes through distribution remapping to get the output. This section is pre-trained using independently trained model weights. We assume that this mapping is generalizable and freezes its weights when training the final model.

\section{How we use augmentation and HWS}
    Taking depthwise Conv as an example, let's assume we have 3 channels for \texttt{MFConv} and 7 channels for original Conv, which should be set up at the beginning and fixed. We will maintain a convolutional weight parameter with 10 channels in our code. We divide the weights of the first 3 channels as targets and calculate them using \texttt{MFConv}. The weights of the remaining 7 channels are divided as the augmented part and calculated using the original Conv.

    At the end of each epoch, we will reorganize the weights of these 10 channels and move the important weights to the first 3 channels. We use the $l1$ norm to evaluate their importance. Since good weights in original Conv may not be good in \texttt{MFConv}, we need HWS to cope with different weight distributions among different operators. The weights of the first 3 channels are first mapped through HWS, then being used for calculation. We will release the mapped result after calculation during training and only save it at the end of training for exportation.

    We ensure the alignment of channels between \texttt{MFConv} so that the exported target model can run independently. The running process of augmented DWConv is shown in Alg. \ref{alg:AugDWConv}. The training process is shown in Alg. \ref{alg:AugTrain}.
    
    \begin{algorithm}[h]
       \caption{AugDWConv}
       \label{alg:AugDWConv}
    \begin{algorithmic}
       \STATE {\bfseries Input:} target\_channel $c_t$, aug\_channel $c_a$, kernel\_size $k$.
       \STATE Weight = $tensor([c_t+c_a,1,k,k])$.
       \IF{Augmented run}
            \STATE $x$: op input. Size $[bs, c_t+c_a, h, w]$
            \STATE $x_{t}=x[:,:c_t,:,:]$
            \STATE $x_{a}=x[:,c_t:,:,:]$
            \STATE $W_t = Weight[:c_t,:,:,:]$
            \STATE $W_t = HWS(W_t)$
            \STATE $W_a = Weight[c_t:,:,:,:]$
            \STATE $out_t = MFConv(x_{t}, W_t, group=c_t)$
            \STATE $out_a = Conv(x_{a}, W_a, group=c_a)$
            \STATE return $cat((out_t,out_a), dim=1)$
        \ELSE
            \STATE $x$: op input. Size $[bs, c_t, h, w]$
            \STATE $W_t = Weight[:c_t,:,:,:]$
            \STATE $W_t = HWS(W_t)$
            \STATE return $MFConv(x, W_t, group=c_t)$
        \ENDIF
       
    \end{algorithmic}
    \end{algorithm}

    \begin{algorithm}[h]
       \caption{Augmented training}
       \label{alg:AugTrain}
       \begin{algorithmic}
       \STATE {\bfseries Input:} supervision parameter $\alpha_1, \alpha_2$
       \STATE $model = AugmentedHybirdModel()$
       \FOR{0,1,... epoch}
        \FOR{$x,label$ in $dataset$}
            \STATE $pred_{target} = model(x, augmented\_run = False)$
            \STATE $pred_{aug} = model(x, augmented\_run = True)$
            \STATE $loss_{target} = criterion(pred_{target}, label)$
            \STATE $loss_{aug} = criterion(pred_{aug}, label)$
            \STATE $loss = \alpha_1 loss_{target} + \alpha_2 loss_{aug}$
            \STATE $loss.backward()$
        \ENDFOR
        \STATE Reorder important weights to target part.
       \ENDFOR
       \STATE Export target part weights.
       \STATE Remap weights by HWS().
       \STATE Build the multiplicaton-free NN.
       \STATE Load exported weight.
       
    \end{algorithmic}
    \end{algorithm}
